# Supplementary material for: The Localized Active Space Method with Unitary Selective Coupled Cluster
Source: arXiv:2404.12927 source file (2024-04-19)
Supplement: Supplementary file 1 [file SI.pdf]

# Supporting Information:

## The Localized Active Space Method with Unitary Selective Coupled Cluster

Abhishek Mitra,<sup>†</sup> Ruhee D’Cunha,<sup>†</sup> Qiaohong Wang,<sup>‡</sup> Matthew R. Hermes,<sup>†</sup>  
Yuri Alexeev,<sup>¶</sup> Stephen K. Gray,<sup>\*,¶</sup> Matthew Otten,<sup>\*,§</sup> and Laura Gagliardi<sup>\*,†,‡,¶</sup>

<sup>†</sup>*Department of Chemistry, Chicago Center for Theoretical Chemistry, University of  
Chicago, Chicago, IL 60637, USA.*

<sup>‡</sup>*Pritzker School of Molecular Engineering, Chicago Center for Theoretical Chemistry,  
University of Chicago, Chicago, IL 60637, USA.*

<sup>¶</sup>*Argonne National Laboratory 9700 S. Cass Avenue Lemont, IL 60439*

<sup>§</sup>*Department of Physics, University of Wisconsin – Madison, Madison, WI 53726, USA.*

E-mail: gray@anl.gov; mjotten@wisc.edu; lgagliardi@uchicago.edu

### S01. Derivation of USCC condition

The Unitary Coupled Cluster wave function can be written as:

$$|\Psi_{\text{UCC}}\rangle = e^{\hat{T}-\hat{T}^\dagger}|\Phi_0\rangle, \quad (1)$$

where  $|\Phi_0\rangle$  denotes the reference (Hartree-Fock) wave function, and  $\hat{T}$  represents the cluster operator encompassing single, double excitations, and higher excitations if required. The

energy can be formulated as:

$$E = \frac{\langle \Phi_0 | e^{\hat{T}^\dagger - \hat{T}} \hat{H} e^{\hat{T} - \hat{T}^\dagger} | \Phi_0 \rangle}{\langle \Phi_0 | e^{\hat{T}^\dagger - \hat{T}} e^{\hat{T} - \hat{T}^\dagger} | \Phi_0 \rangle}, \quad (2)$$

$$\bar{H} = e^{\hat{T}^\dagger - \hat{T}} \hat{H} e^{\hat{T} - \hat{T}^\dagger}, \quad (3)$$

We can define a new variable, the anti-Hermitian operator  $\hat{\tau} = \hat{T} - \hat{T}^\dagger$ , and employ the Baker-Campbell-Hausdorff (BCH) expansion for  $e^{-\hat{\tau}} \hat{H} e^{\hat{\tau}}$ :

$$\bar{H} = e^{-\hat{\tau}} \hat{H} e^{\hat{\tau}} = \hat{H} + [\hat{H}, \hat{\tau}] + \frac{1}{2!} [[\hat{H}, \hat{\tau}], \hat{\tau}] + \frac{1}{3!} [[[ \hat{H}, \hat{\tau} ], \hat{\tau} ], \hat{\tau}] + \dots, \quad (4)$$

Now, considering the wave functions are normalized the UCC energy  $E_{UCC}$  can be written as

$$\begin{aligned} E_{UCC} &= \langle \Phi_0 | \bar{H} | \Phi_0 \rangle = \langle \Phi_0 | \left( e^{-\hat{\tau}} \hat{H} e^{\hat{\tau}} \right) | \Phi_0 \rangle \\ &= \langle \Phi_0 | \left( \hat{H} + [\hat{H}, \hat{\tau}] + \frac{1}{2!} [[\hat{H}, \hat{\tau}], \hat{\tau}] + \frac{1}{3!} [[[ \hat{H}, \hat{\tau} ], \hat{\tau} ], \hat{\tau}] + \dots \right) | \Phi_0 \rangle. \end{aligned} \quad (5)$$

Utilizing this energy equation, we can express the derivative of  $E_{UCC}$  with respect to  $t_i^a$  as:

$$\frac{\partial E_{UCC}}{\partial t_i^a} = \frac{\partial}{\partial t_i^a} \langle \Phi_0 | \left( \hat{H} + [\hat{H}, \hat{\tau}] + \frac{1}{2!} [[\hat{H}, \hat{\tau}], \hat{\tau}] + \dots \right) | \Phi_0 \rangle. \quad (6)$$

This can be further written down as:

$$\begin{aligned} \frac{\partial E_{UCC}}{\partial t_i^a} &= \frac{\partial}{\partial t_i^a} \langle \Phi_0 | \left( \hat{H} \right) | \Phi_0 \rangle \\ &\quad + \frac{\partial}{\partial t_i^a} \langle \Phi_0 | \left( [\hat{H}, \hat{\tau}] \right) | \Phi_0 \rangle \\ &\quad + \frac{\partial}{\partial t_i^a} \langle \Phi_0 | \left( \frac{1}{2!} [[\hat{H}, \hat{\tau}], \hat{\tau}] \right) | \Phi_0 \rangle \\ &\quad + \dots. \end{aligned} \quad (7)$$

Reinserting  $\hat{\tau} = \hat{T} - \hat{T}^\dagger$ , we get,

$$\begin{aligned}
\frac{\partial E_{\text{UCC}}}{\partial t_i^a} &= \frac{\partial}{\partial t_i^a} \langle \Phi_0 | \left( \hat{H} \right) | \Phi_0 \rangle \\
&+ \frac{\partial}{\partial t_i^a} \langle \Phi_0 | \left( [\hat{H}, \hat{T} - \hat{T}^\dagger] \right) | \Phi_0 \rangle \\
&+ \frac{\partial}{\partial t_i^a} \langle \Phi_0 | \left( \frac{1}{2!} [[\hat{H}, \hat{T} - \hat{T}^\dagger], \hat{T} - \hat{T}^\dagger] \right) | \Phi_0 \rangle \\
&+ \dots.
\end{aligned} \tag{8}$$

Using,  $\hat{T} = \hat{T}_1 + \hat{T}_2$

$$\begin{aligned}
\frac{\partial E_{\text{UCC}}}{\partial t_i^a} &= \frac{\partial}{\partial t_i^a} \langle \Phi_0 | \left( \hat{H} \right) | \Phi_0 \rangle \\
&+ \frac{\partial}{\partial t_i^a} \langle \Phi_0 | \left( [\hat{H}, (\hat{T}_1 + \hat{T}_2) - (\hat{T}_1^\dagger + \hat{T}_2^\dagger)] \right) | \Phi_0 \rangle \\
&+ \frac{\partial}{\partial t_i^a} \langle \Phi_0 | \left( \frac{1}{2!} [[\hat{H}, (\hat{T}_1 + \hat{T}_2) - (\hat{T}_1^\dagger + \hat{T}_2^\dagger)], (\hat{T}_1 + \hat{T}_2) - (\hat{T}_1^\dagger + \hat{T}_2^\dagger)] \right) | \Phi_0 \rangle \\
&+ \dots,
\end{aligned} \tag{9}$$

where,

$$\hat{T}_1 = \sum_{i,a} t_i^a \hat{a}_a^\dagger \hat{a}_i, \tag{10}$$

and,

$$\hat{T}_2 = \sum_{i,j,a,b} t_{ij}^{ab} \hat{a}_a^\dagger \hat{a}_b^\dagger \hat{a}_j \hat{a}_i, \tag{11}$$

Let's rewrite the expression for the partial derivative of  $E_{\text{UCC}}$  with respect to  $t_i^a$  using the definitions of  $\hat{T}_1$  and  $\hat{T}_2$ . Although we evaluate the partial derivative at  $t_i^a = 0$ , we intentionally maintain the first term and the  $T_2$  operators to ensure clarity in the expression.

$$\begin{aligned}
\left. \frac{\partial E_{\text{UCC}}}{\partial t_i^a} \right|_{t_i^a=0} &= \frac{\partial}{\partial t_i^a} \langle \Phi_0 | \left( \hat{H} \right) | \Phi_0 \rangle \\
&+ \frac{\partial}{\partial t_i^a} \langle \Phi_0 | \left( [\hat{H}, (\sum_{j,b} t_j^b \hat{a}_b^\dagger \hat{a}_j + \sum_{j,k,b,c} t_{jk}^{bc} \hat{a}_b^\dagger \hat{a}_c^\dagger \hat{a}_k \hat{a}_j) - (\sum_{j,b} t_j^b \hat{a}_j^\dagger \hat{a}_b + \sum_{j,k,b,c} t_{jk}^{bc} \hat{a}_j^\dagger \hat{a}_k^\dagger \hat{a}_c \hat{a}_b)] \right) | \Phi_0 \rangle.
\end{aligned} \tag{12}$$

Since the derivative of the first and all  $\hat{T}_2$  terms with respect to  $t_i^a$  is 0 and  $T_1^\dagger |\Phi_0\rangle = 0$ , we get:

$$\left. \frac{\partial E_{\text{UCC}}}{\partial t_i^a} \right|_{t_i^a=0} = \langle \Phi_0 | \left( [\hat{H}, \hat{a}_a^\dagger \hat{a}_i - \hat{a}_i^\dagger \hat{a}_a] \right) | \Phi_0 \rangle. \quad (13)$$

To further analyze the expression for the partial derivative of  $E_{\text{UCC}}$  with respect to  $t_i^a$ , we can expand the commutator:

$$\frac{\partial E_{\text{UCC}}}{\partial t_i^a} = \langle \Phi_0 | \left( \hat{H} \hat{a}_a^\dagger \hat{a}_i - \hat{a}_a^\dagger \hat{a}_i \hat{H} - \hat{H} \hat{a}_i^\dagger \hat{a}_a + \hat{a}_i^\dagger \hat{a}_a \hat{H} \right) | \Phi_0 \rangle. \quad (14)$$

We can present the expression for the partial derivative of  $E_{\text{UCC}}$  with respect to  $t_i^a$  as:

$$\begin{aligned} \frac{\partial E_{\text{UCC}}}{\partial t_i^a} &= \langle \Phi_0 | \hat{H} \hat{a}_a^\dagger \hat{a}_i | \Phi_0 \rangle \\ &\quad - \langle \Phi_0 | \hat{a}_a^\dagger \hat{a}_i \hat{H} | \Phi_0 \rangle \\ &\quad - \langle \Phi_0 | \hat{H} \hat{a}_i^\dagger \hat{a}_a | \Phi_0 \rangle \\ &\quad + \langle \Phi_0 | \hat{a}_i^\dagger \hat{a}_a \hat{H} | \Phi_0 \rangle. \end{aligned} \quad (15)$$

Considering that  $\Phi_0$  is a Hartree-Fock determinant,  $i$  represents occupied orbitals, and  $a$  represents virtual orbitals, we can simplify the expression for the partial derivative of  $E_{\text{UCC}}$  with respect to  $t_i^a$  as follows:

$$\begin{aligned} \left. \frac{\partial E_{\text{UCC}}}{\partial t_i^a} \right|_{t_i^a=0} &= \langle \Phi_0 | \hat{H} \hat{a}_a^\dagger \hat{a}_i | \Phi_0 \rangle \\ &\quad + \langle \Phi_0 | \hat{a}_i^\dagger \hat{a}_a \hat{H} | \Phi_0 \rangle. \end{aligned} \quad (16)$$

Let's rewrite the expression for the partial derivative of  $E_{\text{UCC}}$  with respect to  $t_i^a$  in terms of  $\Phi_i^a$ . Since  $\hat{a}_a^\dagger \hat{a}_i |\Phi_0\rangle = |\Phi_i^a\rangle$ , we have:

$$\begin{aligned} \frac{\partial E_{\text{UCC}}}{\partial t_i^a} &= \langle \Phi_0 | \hat{H} | \Phi_i^a \rangle \\ &+ \langle \Phi_i^a | \hat{H} | \Phi_0 \rangle, \end{aligned} \quad (17)$$

$$\frac{\partial E_{\text{UCC}}}{\partial t_i^a} = 2 \langle \Phi_0 | \hat{H} | \Phi_i^a \rangle. \quad (18)$$

Now, let's denote  $\langle \Phi_0 | \hat{H} | \Phi_i^a \rangle$  as  $H_i^a$ :

$$\frac{\partial E_{\text{UCC}}}{\partial t_i^a} = 2H_i^a = 2H_{ia}. \quad (19)$$

Similarly, it can be shown that:

$$\frac{\partial E_{\text{UCC}}}{\partial t_{ij}^{ab}} = 2H_{ij}^{ab}. \quad (20)$$

The compound index  $\beta$  is used to signify both  $i \rightarrow a$  and  $i, j \rightarrow a, b$  excitations.

### Proposed USCC conditions

Equation (21) is now used to select the  $t_i^a$  and  $t_{ij}^{ab}$  amplitudes for the first VQE iteration:

$$|H_{\beta 0}| = \left| \frac{\partial E_{\text{UCC}}}{\partial t_\beta} \right|_{t_\beta=0} \geq \epsilon. \quad (21)$$

## S02. Convergence of LAS-USCCSD for $\text{Cr}_2(\text{OH})_3(\text{NH}_3)_6]^{3+}$

The VQE step for the LAS-USCCSD algorithm is performed using the L-BFGS-B Scipy optimizer. We plot the projected gradient of the function being optimized which has the default value of  $10^{-5}$ . While LAS-USCCSD using 12 and 77 parameters converge, the projected gradient values of the LAS-UCCSD is still at  $10^{-3}$  after 240 hours of runtime and requires further time for convergence.

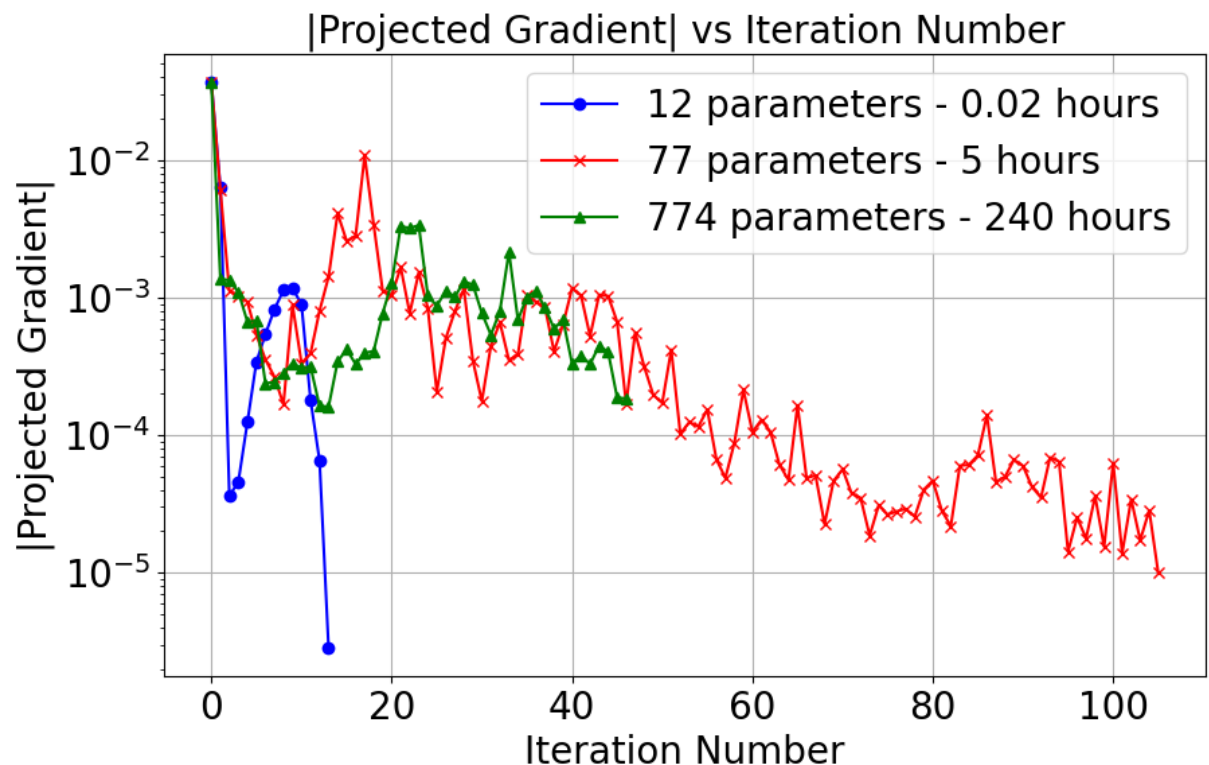

Figure S1: The projected gradient value for the L-BFGS-B optimizer computed using LAS-USCCSD (12 and 77 parameters) and LAS-UCCSD method (774 parameters) for  $\text{Cr}_2(\text{OH})_3(\text{NH}_3)_6]^{3+}$ .

### S03. Total Energies

The operator ordering for all the energies can be viewed in the GitHub repository used to generate all the converged energies.<sup>S1</sup> Particularly, the most important parameters are selected using the `get_grad.t1` function located in the path

LAS-USCC/mrh-4-uscc/mrh/exploratory/citools/lasci\_ominus1.py.

Table S1: Dependence of the number of parameters on  $\epsilon$  and the corresponding total energies for the  $H_4$  system at  $R = 1.46 \text{ \AA}$

| $\epsilon$ | Parameters | LAS-USCCSD Energy (Ha) |
|------------|------------|------------------------|
| 0.100000   | 0          | -2.102636              |
| 0.062506   | 4          | -2.103902              |
| 0.009541   | 14         | -2.106346              |
| 0.007543   | 23         | -2.107519              |
| 0.005964   | 26         | -2.108738              |
| 0.004715   | 28         | -2.108741              |
| 0.002947   | 32         | -2.108741              |
| 0.001456   | 36         | -2.108741              |
| 0.000910   | 38         | -2.108741              |
| 0.000087   | 40         | -2.108741              |

Table S2: Dependence of the number of parameters on  $\epsilon$  and the corresponding total energies for the  $H_4$  system at  $R = 0.96 \text{ \AA}$

| $\epsilon$ | Parameters | LAS-USCCSD Energy (Ha) |
|------------|------------|------------------------|
| 0.100000   | 4          | -1.792223              |
| 0.027295   | 5          | -1.792265              |
| 0.026519   | 7          | -1.797220              |
| 0.025765   | 11         | -1.813979              |
| 0.022956   | 19         | -1.865929              |
| 0.021053   | 20         | -1.869365              |
| 0.018758   | 28         | -1.909591              |
| 0.016238   | 30         | -1.910627              |
| 0.010533   | 34         | -1.910626              |
| 0.006638   | 36         | -1.910627              |
| 0.001976   | 40         | -1.910627              |

Table S3: Dependence of the number of parameters on  $\epsilon$  and the corresponding total energies for the  $H_8$

| Epsilon  | Parameters | LAS-USCCSD Energy |
|----------|------------|-------------------|
| 1.00e-01 | 0          | -4.087716         |
| 6.89e-02 | 2          | -4.088721         |
| 5.72e-02 | 12         | -4.091341         |
| 1.87e-02 | 13         | -4.091370         |
| 1.56e-02 | 29         | -4.093114         |
| 1.29e-02 | 33         | -4.094243         |
| 1.07e-02 | 41         | -4.095697         |
| 8.90e-03 | 89         | -4.100330         |
| 7.39e-03 | 110        | -4.103073         |
| 6.14e-03 | 114        | -4.104720         |
| 5.09e-03 | 136        | -4.106304         |
| 3.51e-03 | 146        | -4.106913         |
| 2.92e-03 | 182        | -4.107107         |
| 2.42e-03 | 206        | -4.107421         |
| 2.01e-03 | 237        | -4.107900         |
| 1.67e-03 | 269        | -4.108089         |
| 1.38e-03 | 303        | -4.109194         |
| 1.15e-03 | 333        | -4.109283         |
| 9.55e-04 | 347        | -4.109488         |
| 5.46e-04 | 398        | -4.110002         |
| 4.53e-04 | 409        | -4.110013         |
| 3.76e-04 | 441        | -4.110463         |
| 3.13e-04 | 449        | -4.110497         |
| 2.60e-04 | 475        | -4.110891         |
| 2.15e-04 | 486        | -4.110852         |
| 1.79e-04 | 492        | -4.110857         |
| 1.48e-04 | 508        | -4.110918         |
| 1.23e-04 | 524        | -4.110982         |
| 1.02e-04 | 533        | -4.111059         |
| 8.50e-05 | 538        | -4.111083         |
| 7.05e-05 | 544        | -4.111114         |
| 5.86e-05 | 546        | -4.111109         |
| 4.04e-05 | 548        | -4.111115         |
| 2.78e-05 | 552        | -4.111116         |
| 2.31e-05 | 556        | -4.111102         |
| 1.92e-05 | 562        | -4.111159         |

Table S4: Dependence of the number of parameters on  $\epsilon$  and the corresponding total energies for the  $H_8$

| Epsilon  | Parameters | LAS-USCCSD Energy |
|----------|------------|-------------------|
| 7.56e-06 | 564        | -4.111162         |
| 4.64e-07 | 580        | -4.111168         |
| 3.85e-07 | 588        | -4.111175         |
| 2.21e-07 | 590        | -4.111180         |
| 1.83e-07 | 594        | -4.111205         |
| 1.52e-07 | 604        | -4.111206         |
| 1.26e-07 | 626        | -4.111207         |
| 1.05e-07 | 638        | -4.111209         |
| 8.70e-08 | 686        | -4.111212         |
| 7.22e-08 | 742        | -4.111219         |
| 5.99e-08 | 780        | -4.111222         |
| 4.98e-08 | 828        | -4.111221         |
| 4.13e-08 | 872        | -4.111226         |
| 3.43e-08 | 910        | -4.111227         |
| 2.85e-08 | 932        | -4.111221         |
| 2.36e-08 | 994        | -4.111234         |
| 1.96e-08 | 1026       | -4.111237         |
| 1.63e-08 | 1074       | -4.111238         |
| 1.35e-08 | 1122       | -4.111240         |
| 1.12e-08 | 1218       | -4.111243         |
| 9.33e-09 | 1302       | -4.111240         |
| 7.74e-09 | 1372       | -4.111245         |
| 6.43e-09 | 1450       | -4.111242         |
| 5.34e-09 | 1504       | -4.111245         |
| 4.43e-09 | 1560       | -4.111246         |
| 3.68e-09 | 1650       | -4.111247         |
| 3.05e-09 | 1704       | -4.111244         |
| 2.54e-09 | 1756       | -4.111248         |
| 2.10e-09 | 1800       | -4.111247         |
| 1.75e-09 | 1850       | -4.111246         |
| 1.45e-09 | 1888       | -4.111249         |
| 1.20e-09 | 1914       | -4.111244         |
| 1.00e-09 | 1988       | -4.111249         |

Table S5: Dependence of the number of parameters on  $\epsilon$  and the corresponding total energies for the *trans*-butadiene geometry 1

| Epsilon  | LAS-USCCSD Energy | Parameters |
|----------|-------------------|------------|
| 3.61e-02 | -154.972815       | 0          |
| 2.34e-02 | -154.973125       | 2          |
| 1.52e-02 | -154.973601       | 44         |
| 1.22e-02 | -154.973769       | 52         |
| 7.93e-03 | -154.975197       | 56         |
| 6.39e-03 | -154.976197       | 68         |
| 5.14e-03 | -154.976245       | 76         |
| 4.14e-03 | -154.976257       | 84         |
| 2.69e-03 | -154.976297       | 100        |
| 2.16e-03 | -154.976358       | 124        |
| 1.74e-03 | -154.976386       | 170        |
| 1.13e-03 | -154.976394       | 190        |
| 9.10e-04 | -154.976417       | 200        |
| 7.33e-04 | -154.976437       | 212        |
| 5.90e-04 | -154.976448       | 232        |
| 3.83e-04 | -154.976450       | 238        |
| 2.48e-04 | -154.976450       | 240        |
| 1.04e-04 | -154.976450       | 242        |
| 4.65e-07 | -154.976450       | 244        |
| 3.02e-07 | -154.976449       | 248        |
| 1.58e-07 | -154.976451       | 260        |
| 1.27e-07 | -154.976450       | 266        |
| 1.02e-07 | -154.976459       | 278        |
| 8.23e-08 | -154.976458       | 288        |
| 6.63e-08 | -154.976459       | 296        |
| 5.34e-08 | -154.976460       | 314        |
| 4.30e-08 | -154.976489       | 350        |
| 3.46e-08 | -154.976492       | 366        |
| 2.79e-08 | -154.976491       | 384        |
| 2.24e-08 | -154.976493       | 424        |
| 1.46e-08 | -154.976495       | 456        |
| 1.17e-08 | -154.976494       | 472        |
| 9.44e-09 | -154.976496       | 484        |
| 7.60e-09 | -154.976496       | 492        |
| 6.12e-09 | -154.976497       | 528        |
| 4.93e-09 | -154.976497       | 548        |
| 3.97e-09 | -154.976495       | 560        |
| 3.20e-09 | -154.976500       | 588        |
| 2.57e-09 | -154.976497       | 596        |
| 1.67e-09 | -154.976501       | 604        |
| 8.72e-10 | -154.976496       | 608        |

Table S6: Dependence of the number of parameters on  $\epsilon$  and the corresponding total energies for the *trans*-butadiene geometry 2

| $\epsilon$   | Parameters | LAS-USCCSD Energy (Ha) |
|--------------|------------|------------------------|
| 1.295574e-01 | 0          | -154.417006            |
| 8.221000e-02 | 96         | -154.511497            |
| 3.310162e-02 | 128        | -154.554755            |
| 1.371151e-03 | 159        | -154.554699            |
| 8.700571e-04 | 224        | -154.562049            |
| 5.842963e-06 | 288        | -154.563038            |
| 3.814231e-07 | 290        | -154.563048            |
| 2.420301e-07 | 292        | -154.563052            |
| 1.061032e-10 | 296        | -154.563053            |
| 1.872891e-14 | 520        | -154.563047            |
| 1.577940e-24 | 584        | -154.563269            |

Table S7: Dependence of the number of parameters on  $\epsilon$  and the corresponding total energies for the low spin ground state for tris-( $\mu$ -hydroxo)-bridged chromium compound

| Epsilon  | Parameters | LAS-USCCSD Energy (Ha) |
|----------|------------|------------------------|
| 8.50e-02 | 0          | -2649.144940           |
| 2.31e-02 | 12         | -2649.145916           |
| 7.39e-03 | 36         | -2649.146006           |
| 1.05e-03 | 60         | -2649.146016           |
| 1.48e-04 | 61         | -2649.146016           |
| 1.07e-04 | 63         | -2649.146016           |
| 7.74e-05 | 67         | -2649.146017           |
| 3.43e-05 | 77         | -2649.146145           |
| 2.48e-05 | 79         | -2649.146145           |
| 1.79e-05 | 99         | -2649.146145           |
| 1.52e-05 | 121        | -2649.146145           |
| 1.10e-05 | 129        | -2649.146145           |
| 9.33e-06 | 137        | -2649.146140           |
| 7.92e-06 | 147        | -2649.146145           |
| 6.73e-06 | 159        | -2649.146145           |
| 5.72e-06 | 163        | -2649.146145           |
| 2.15e-06 | 183        | -2649.146163           |
| 5.86e-07 | 187        | -2649.146164           |
| 1.15e-07 | 189        | -2649.146163           |
| 5.09e-08 | 191        | -2649.146163           |
| 3.68e-08 | 193        | -2649.146163           |
| 2.66e-08 | 195        | -2649.146161           |

## S04. LAS-UCCSD Gradient implementation

In the current implementation, the unitary  $\hat{U}_{\text{UCCSD}}$  is expressed in the form of a first-order Trotterization as:

$$\hat{U}_{\text{UCCSD}} = U = U_0.U_1.U_2... \quad (22)$$

so that the expression

$$\langle \Psi | U H U' | \Psi \rangle = \langle \bigwedge_K (\Psi_{A_K}) | U H U' | \bigwedge_K (\Psi_{A_K}) \rangle \quad (23)$$

is differentiated as

$$\langle \Psi | dU_0.U_1.U_2...H.U' | \Psi \rangle + \langle \Psi | U_0.dU_1.U_2...H.U' | \Psi \rangle + \langle \Psi | U_0.U_1.dU_2...H.U' | \Psi \rangle + ... \quad (24)$$

where each  $U$  factor depends on the  $t$  amplitudes, and no assumptions are made about the value of the  $t$  amplitudes about which the differentiation is carried out. Here  $|\Psi\rangle = |\Psi_{\text{QLAS}}\rangle = \bigwedge_K (\Psi_{A_K})$  and therefore has no explicit dependence on  $t$ . However, even though we do not perform any LAS-UCCSD iteration step, storing  $t$  amplitudes require memory. Here, we show that the gradients can be constructed classically in a more memory efficient way, since in practice we only requires gradients evaluated at the origin,  $\mathbf{t} = 0$ . The gradients can be written generally as:

$$\left. \frac{\partial E_{\text{LAS-UCCSD}}}{\partial t_\beta} \right|_{\mathbf{t}=0} = \langle \Psi | [\hat{H}, a_\beta] | \Psi \rangle - \langle \Psi | [\hat{H}, a_\beta^\dagger] | \Psi \rangle \quad (25)$$

The full expression for the gradients will have  $h_1 t_1$ ,  $h_2 t_1$ ,  $h_1 t_2$  and  $h_2 t_2$  terms. For simplicity, we only show how the  $h_1 t_1$  terms can be constructed. The rest of the terms can be similarly constructed. Let  $u, v, w, x, y$  be general indices

$$\frac{\partial E_{\text{LAS-UCC}}}{\partial t_x^u} = \langle \Psi | \hat{H} \hat{a}_u^\dagger \hat{a}_x | \Psi \rangle - \langle \Psi | \hat{a}_u^\dagger \hat{a}_x \hat{H} | \Psi \rangle - \langle \Psi | \hat{H} \hat{a}_x^\dagger \hat{a}_u | \Psi \rangle + \langle \Psi | \hat{a}_x^\dagger \hat{a}_u \hat{H} | \Psi \rangle \quad (26)$$

Again, we only consider the first term only since the others will have the same properties.

We know:

$$\hat{\hat{H}} = \sum_{pq} h_{pq} \hat{a}_p^\dagger \hat{a}_q + \frac{1}{2} \sum_{pqrs} \langle pq || rs \rangle \hat{a}_p^\dagger \hat{a}_q^\dagger \hat{a}_s \hat{a}_r \quad (27)$$

and let the first term  $\text{FT}_{h_1 t_1}$  be

$$\text{FT}_{h_1 t_1} = \sum_{pq} h_{pq} \langle \Psi | \hat{a}_p^\dagger \hat{a}_q \hat{a}_u^\dagger \hat{a}_x | \Psi \rangle = \sum_{pq} h_{pq} \langle \Psi | a_q^p a_x^u | \Psi \rangle \quad (28)$$

Before we show this, from Kong et al,<sup>S2</sup> the density matrices and cumulants for an arbitrary wave function  $\Psi$  can be expressed as:

$$\gamma_q^p \equiv \langle \Psi | a_q^p | \Psi \rangle, \quad (29)$$

$$\gamma_{qs}^{pr} \equiv \langle \Psi | a_{qs}^{pr} | \Psi \rangle, \quad (30)$$

$$\gamma_{q \dots s}^{p \dots r} \equiv \langle \Psi | a_{q \dots s}^{p \dots r} | \Psi \rangle \quad (31)$$

and cumulants

$$\gamma_q^p \equiv \lambda_q^p, \quad (32)$$

$$\gamma_{qs}^{pr} \equiv \lambda_{qs}^{pr} + \lambda_q^p \lambda_s^r - \lambda_s^p \lambda_q^r = \lambda_{qs}^{pr} + \mathcal{A}(\lambda_q^p \lambda_s^r), \quad (33)$$

$$\gamma_{qsu}^{prt} \equiv \lambda_{qsu}^{prt} + \mathcal{A}(\lambda_q^p \lambda_s^r \lambda_u^t + \lambda_q^p \lambda_{su}^{rt}). \quad (34)$$

From reference S3, it can be shown that

$$\begin{aligned}
\text{FT}_{h_1 t_1} &= \sum_{pq} h_{pq} \langle \Psi | \tilde{a}_q^p \tilde{a}_x^u | \Psi \rangle + \gamma_x^u \langle \Psi | \tilde{a}_q^p | \Psi \rangle + \gamma_q^p \langle \Psi | \tilde{a}_x^u | \Psi \rangle + \gamma_q^p \gamma_x^u \langle \Psi | | \Psi \rangle \\
&= \sum_{pq} h_{pq} \langle \Psi | (\tilde{a}_{qx}^{pu} + \eta_q^u \tilde{a}_x^p - \gamma_x^p \tilde{a}_q^u + \eta_q^u \gamma_x^p + \gamma_{qx}^{pu} - \gamma_q^p \gamma_x^u + \gamma_q^u \gamma_x^p) | \Psi \rangle \\
&\quad + \gamma_x^u \langle \Psi | \tilde{a}_q^p | \Psi \rangle + \gamma_q^p \langle \Psi | \tilde{a}_x^u | \Psi \rangle + \gamma_q^p \gamma_x^u \langle \Psi | | \Psi \rangle) \\
&= \sum_{pq} h_{pq} (\langle \Psi | \tilde{a}_{qx}^{pu} | \Psi \rangle + \eta_q^u \langle \Psi | \tilde{a}_x^p | \Psi \rangle - \gamma_x^p \langle \Psi | \tilde{a}_q^u | \Psi \rangle + \eta_q^u \gamma_x^p \langle \Psi | | \Psi \rangle) \\
&\quad + \gamma_{qx}^{pu} \langle \Psi | | \Psi \rangle - \gamma_q^p \gamma_x^u \langle \Psi | | \Psi \rangle + \gamma_q^u \gamma_x^p \langle \Psi | | \Psi \rangle) \\
&\quad + \gamma_x^u \langle \Psi | \tilde{a}_q^p | \Psi \rangle + \gamma_q^p \langle \Psi | \tilde{a}_x^u | \Psi \rangle + \gamma_q^p \gamma_x^u \langle \Psi | | \Psi \rangle) \\
&= \sum_{pq} h_{pq} (\eta_q^u \gamma_x^p + \gamma_{qx}^{pu} + \gamma_q^u \gamma_x^p)
\end{aligned} \tag{35}$$

Here,  $a_q^p = \tilde{a}_q^p + \gamma_q^p$  where  $a_q^p = a^p a_q$ ,  $\eta_q^p = \delta_q^p - \gamma_q^p$ . Note that  $\langle \Psi | | \Psi \rangle$  is the normalization condition of the state  $\Psi$ , and is typically equal to one. In the last step of the equation, we have used the fact that all expectation values with respect to normal-ordered operators go to 0 as was proven in equations 33a to 33c in reference S3. Similarly, the second term  $\text{ST}_{h_1 t_1}$  can be written as:

$$\begin{aligned}
\text{ST}_{h_1 t_1} &= \sum_{pq} h_{pq} (\langle \Psi | \tilde{a}_x^u \tilde{a}_q^p | \Psi \rangle + \gamma_q^p \langle \Psi | \tilde{a}_x^u | \Psi \rangle + \gamma_x^u \langle \Psi | \tilde{a}_q^p | \Psi \rangle + \gamma_x^u \gamma_q^p \langle \Psi | | \Psi \rangle) \\
&= \sum_{pq} h_{pq} (\eta_x^p \gamma_q^u + \gamma_{xq}^{up} + \gamma_x^p \gamma_q^u)
\end{aligned} \tag{36}$$

Finally, adding the four terms we get:

$$\text{Final}_{h_1 t_1} = \sum_{pq} h_{pq} (\eta_q^u \gamma_x^p + \gamma_{qx}^{pu} + \gamma_q^u \gamma_x^p - \eta_x^p \gamma_q^u - \gamma_{xq}^{up} - \gamma_x^p \gamma_q^u - \tag{37}$$

$$\eta_q^x \gamma_u^p - \gamma_{qu}^{px} - \gamma_q^x \gamma_u^p + \eta_u^p \gamma_q^x + \gamma_{uq}^{xp} + \gamma_u^p \gamma_q^x) \tag{38}$$

In the spinorbital basis, the operator products  $a$ , the normal-ordered operator products  $\tilde{a}$ , the density matrices  $\gamma$ , and the cumulants  $\lambda$  are all antisymmetric upon permutation of any two superscript or any two subscript indices. Thus, all the two-body cumulants cancel since  $\gamma_{qx}^{pu} = \gamma_{qx}^{pu}$ . Thus the final expression reduces to:

$$\begin{aligned} \text{Final}_{h_1 t_1} &= \sum_{pq} h_{pq} ((\eta_q^u + \gamma_q^u) \gamma_x^p - (\eta_x^p + \gamma_x^p) \gamma_q^u - (\eta_q^x + \gamma_q^x) \gamma_u^p + (\eta_u^p + \gamma_u^p) \gamma_q^x) \\ &= \sum_{pq} h_{pq} (\delta_{uq} \gamma_x^p - \delta_{px} \gamma_q^u - \delta_{xq} \gamma_u^p + \delta_{pu} \gamma_q^x) \end{aligned} \quad (39)$$

The density matrix elements which appear in Eq. (39) are nonzero only for both indices belonging to a single fragment. Recall  $\mathbf{t} = 0$  and  $|\Psi\rangle = |\Psi_{\text{QLAS}}\rangle = \bigwedge_K (\Psi_{A_K})$  since  $\mathbf{t} = 0$ . As an example, the one-body cumulant can be written as:

$$\gamma_q^p \equiv \langle \bigwedge_K (\Psi_{A_K}) | a_q^p | \bigwedge_K (\Psi_{A_K}) \rangle \quad (40)$$

Assuming there are two fragments K and L only

$$\gamma_q^p \equiv \langle (\Psi_{A_K} \otimes \Psi_{A_L}) | a_q^p | (\Psi_{A_K} \otimes \Psi_{A_L}) \rangle \quad (41)$$

The cumulants ( $\lambda$ ) are identically zero unless all spinorbital indices belong to the same fragment, since any term of the type  $\langle (\Psi_{A_K}) | a_q^p | (\Psi_{A_L}) \rangle$  vanishes due to the orthogonality of the different fragments' active subspaces. The same is true of 2-body and 3-body cumulants because the only nonzero 2- and 3-RDM elements are those for which the operator  $a_{q\dots s}^{p\dots r}$  factorizes into a product of operators for different fragments, and the cumulant is defined as the difference between the density matrix and just such a factorized product.

While the  $h_1 t_1$  terms only depend on the one-body cumulants, the final gradient can be shown to depend on one, two and three-body cumulants. Therefore, the final programmable equations will include 1-RDMs, 2-RDMs, and 3-RDMs for the whole system which can be

assembled from the RDMs of the individual fragments resulting in memory requirements only of the order of a LASSCF calculation.

#### S05. LASSCF orbitals for $H_4$

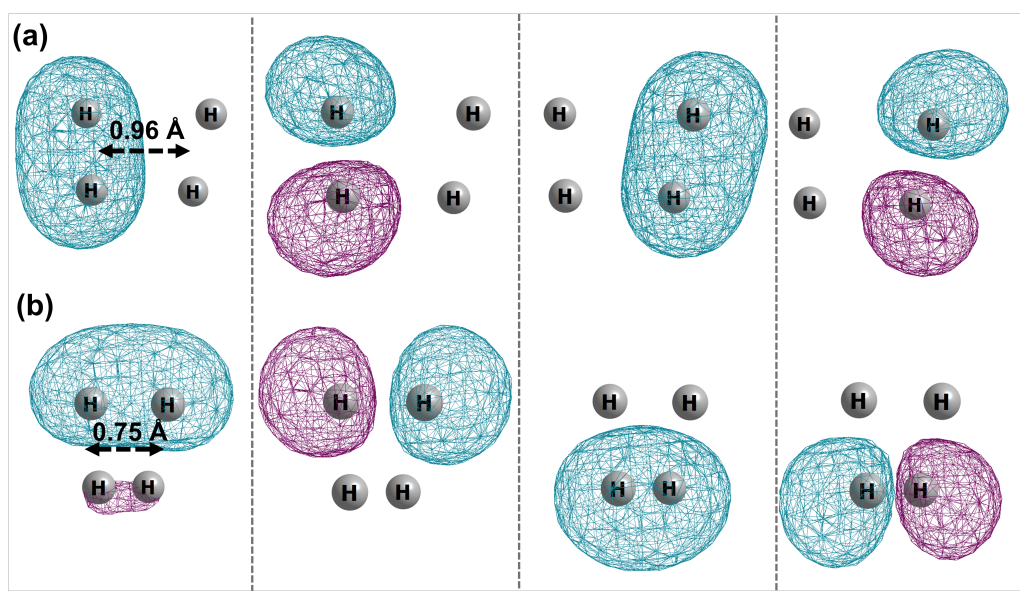

Figure S2: (a) LASSCF orbitals for the  $H_4$  molecule at an inter-fragment distance of 0.96 Å. (b) LASSCF orbitals for the  $H_4$  molecule at an inter-fragment distance of 0.75 Å.

## References

- (S1) Mitra, A. LAS-USCC: A code to perform localized active space unitary selected coupled cluster calculations. 2023; <https://github.com/mitra054/LAS-USCC>, accessed January, 29, 2024.
- (S2) Kong, L.; Nooijen, M.; Mukherjee, D. An algebraic proof of generalized Wick theorem. *J. Chem. Phys.* **2010**, *132*.
- (S3) Kutzelnigg, W.; Mukherjee, D. Normal order and extended Wick theorem for a multi-configuration reference wave function. *J. Chem. Phys.* **1997**, *107*, 432–449.
